# Supplementary material for: Direct Transport between Superconducting Subgap States in a Double Quantum Dot
Source: arXiv:2105.06815 ancillary file (2021-05-14)
Supplement: Supplementary file 1 [file SupplementaryMaterial.pdf]

# Supplementary Information
# Direct Transport between Superconducting Subgap States in a Double Quantum Dot

G. O. Steffensen,[1] J. C. Estrada Saldaña,[1] A. Vekris,[1,2] P. Krogstrup,[1,3]
K. Grove-Rasmussen,[1] J. Nygård,[1] A. L. Yeyati,[4] and J. Paaske[1]

[1] *Center for Quantum Devices, Niels Bohr Institute, University of Copenhagen, 2100 Copenhagen, Denmark*

[2] *Sino-Danish College (SDC), University of Chinese Academy of Sciences*

[3] *Microsoft Quantum Materials Lab Copenhagen, Niels Bohr Institute, University of Copenhagen, 2100 Copenhagen, Denmark*

[4] *Departamento de Física Teórica de la Materia Condensada, Condensed Matter Physics Center (IFIMAC), and Instituto Nicolás Cabrera, Universidad Autónoma de Madrid, 28049 Madrid, Spain*

**CONTENTS**

S1. Experimental details S2
 A. Parameter extraction S2
 B. Zero-bias conductance S2

S2. Floquet Green functions S4
 A. Low bias features S9
 B. Multigap model S10

S3. Master Equations for subgap state transport S11
 A. Conductance asymmetry S14
 B. Singlet-to-doublet Master Equations S15

References S21

## S1. EXPERIMENTAL DETAILS

### A. Parameter extraction

We obtain the charging energies, $U_L$ and $U_R$, from Coulomb-diamond spectroscopy. The data, shown in Fig. S1, were taken in the same shell as those shown in the main article, but for a slightly different gate configuration, which corresponds to the zero-bias differential conductance colormap shown in Fig. S1 (a), through which gates 2 and 4 were swept to obtain the Coulomb diamond plots for both quantum dots in the superconducting state. This change in gate configuration was done to reduce the coupling of the left quantum dot to the left lead, and thereby obtain sharper Coulomb diamonds. The charging energies are given by the distance in bias voltage between the edge of the superconducting gap and the apex of the central diamond in Figs. S1 (b,c) and they correspond to $U_L \approx U_R \approx 2$ meV.

The superconducting gap is extracted using the same gate setting as in the main text, focusing on the nearly gate independent lowermost conductance peak right outside the $eV = E_L + E_R$ feature in Fig. S1 (d). These lines are due to transport between subgap state and opposing gap at $eV = E_{L/R} + \Delta_{R/L}$. At the gate voltage where $eV = E_L + E_R = 0$, we infer that $E_L = E_R = 0$ and read off the values $\Delta_L \approx \Delta_R \approx 0.14$ meV directly from these peak positions (for positive and negative $V$, respectively).

### B. Zero-bias conductance

In Fig. 2 (b) of the main text, we showed zero-bias conductance in a logarithmic scale versus gate voltages 2 and 4. In that diagram, the horizontal features are noted to be sixty times fainter than the vertical features. The faint features cannot be distinguished in the data in Fig. 3 of the main text, as their conductance is too small for the color scale shown there. In Fig. S2, we show differential conductance colormaps which correspond to low-bias versions of Fig. 3 of the main text, with adjusted color scales to highlight the faint features. A zero-bias peak traverses all colormaps, which we attribute to a dissipative supercurrent, as discussed in previous papers [1, 2]. This zero-bias feature is visible is all subplots except (b) where the scale is set by the $eV = E_L + E_R$ which continues to zero bias. The dissipative supercurrent peak is only one component of the zero-bias conductance in Fig. 2 (b) of the main text. A second component comes from the crossing of low-bias replica of the subgap

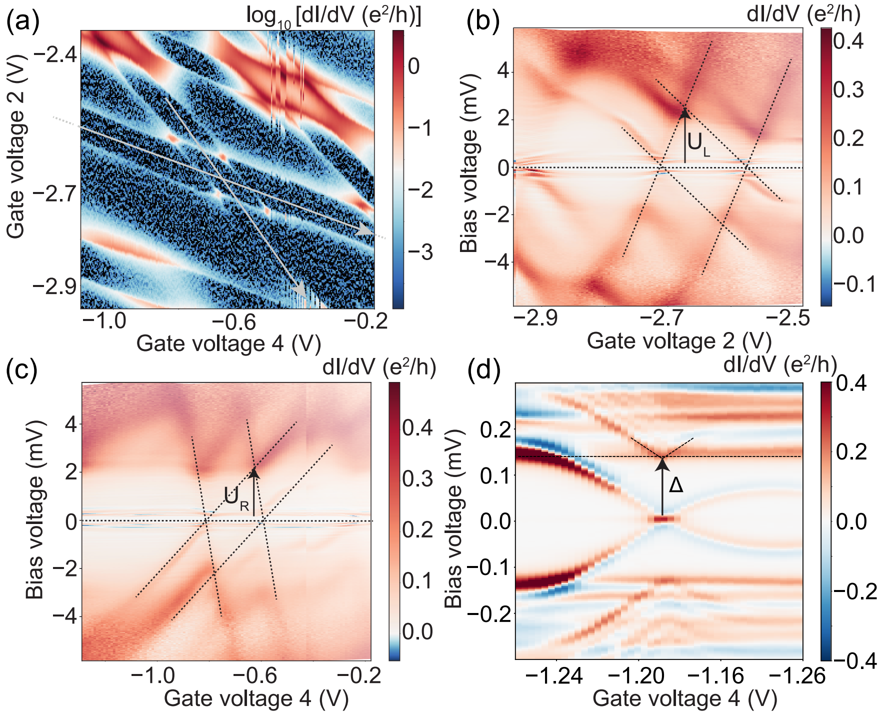


FIG. S1. (a) Colormap of zero-bias differential conductance in logarithmic scale versus gates 2 and 4, with gates 1, 3, 5 set at -9.2 V, -9 V, and -0.36 V, respectively, and the backgate set at 10.4 V. Arrows show gate sweep trajectories in (b) and (c). (b,c) Colormaps of differential conductance versus bias voltage and gate voltage representing Coulomb-diamond spectroscopy of each quantum dot, with the other quantum dot conducting in series in cotunnelling. Dashed lines are drawn on top of the diamonds as a guide to the eye, with the same slope as higher bias features. (d) Colormap of differential conductance versus bias and gate voltage following half the range of linecut 2 in Fig. 3 in the main text. Dotted lines indicate $eV = \Delta_{L/R} + E_{R/L}$ features.

states, which are too faint to be seen in Fig. 3 of the main text but clearly visible in Figs. S2 (a-f). We associate these low-bias replicas with transport between the subgap state and a small residual metallic density of states in the superconducting Al leads, which is consistent with our modelling, as demonstrated below in subsection S2 A.

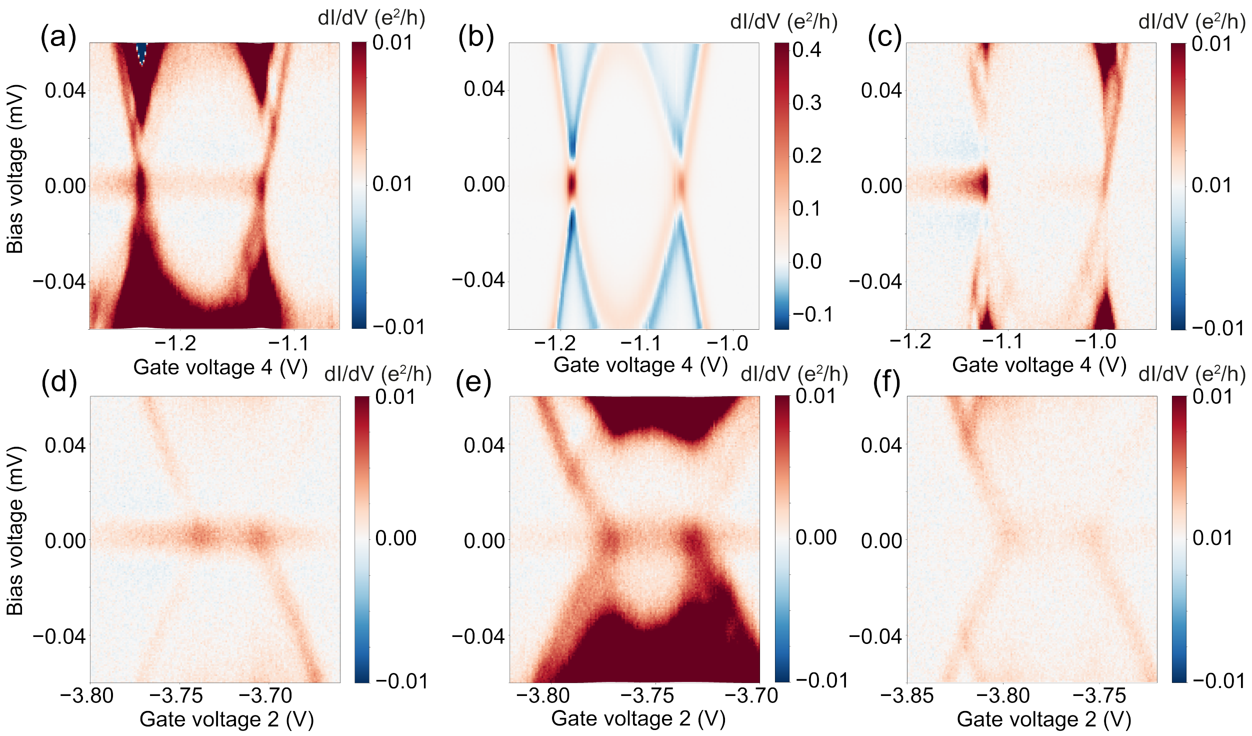


FIG. S2. (a-f) Colormaps of differential conductance versus bias voltage taken through the same gate trajectories as in Fig. 3 of the main text, but with a much reduced bias voltage range.

## S2. FLOQUET GREEN FUNCTIONS

In this section we detail the Floquet Green function calculation underlying the results shown in Fig. 4 in the main text. The Green functions need to include tunnelling to all orders, since the relaxation rate of the subgap states is a small parameter compared to tunneling [3, 4]. Additionally, to capture the Andreev mediated relaxation channels utilizing the opposing gap, our model is required to include multiple Andreev reflections, which is done using a Floquet representation [5]. The derivations presented here are similar to those of Ref. [6, 7].

To describe the interaction between the superconductor and the quantum dot, we utilize a non-self-consistent spin-polarized mean field approximation in which the charging energy, $U$, is replaced by an effective magnetic field $B = U/2$ [6, 8]. Whereas this approximation omits dynamical spin-flips of the dot spin (and hence Kondo-correlations) altogether, it is known to correctly capture many aspects of YSR states [9]. Importantly, this approximation incorrectly describes the odd-parity ground state of the dot-superconductor system as a

singlet state. As we discuss below in section S3 B, this does affect the relaxational transport cycles, albeit in a manner which only leads to quantitative differences in the relaxation rates that one might attempt to infer from a transport experiment. Furthermore, since the mean-field approximation causes the odd-parity singlet state to be spin-polarized, some ground state configurations would show artificial spin blockade. To circumvent this, we choose the magnetic mean fields on each dot to be orthogonal, such that transport occurs via projections between orthogonal spin-spaces allowing transport in all ground state configurations [7].

With these considerations in mind, we write up the Hamiltonian in 4x4 Nambu space, using spinors $\Psi^\dagger_{ik} = \left(c^\dagger_{ki\uparrow}, c^\dagger_{ki\downarrow}, c_{-ki\downarrow}, -c_{-ki\uparrow}\right)$ and $\Phi^\dagger_i = \left(d^\dagger_{i\uparrow}, d^\dagger_{i\downarrow}, d_{i\downarrow}, -d_{i\uparrow}\right)$ for leads and dots respectively with $i \in \{L, R\}$,

$$\begin{aligned}
H &= H_s + H_d + H_{st} + H_{dt} \qquad (1)\\
H_s &= \frac{1}{2}\sum_{i=L,R}\sum_k \Psi^\dagger_{ik}\left(\left(\xi_k - \mu_i\right)\tau_z + \Delta_i\tau_x\right)\Psi_{ik}\\
H_d &= \frac{1}{2}\Phi^\dagger_L\left((\epsilon_L - \mu_L)\tau_z + B_L\sigma_z\right)\Phi_L + \frac{1}{2}\Phi^\dagger_R\left((\epsilon_R - \mu_R)\tau_z + B_R\sigma_x\right)\Phi_R\\
H_{st} &= \frac{1}{2}\sum_{i=L,R}\sum_k t_i\Psi^\dagger_{ik}\tau_z\Phi_i + \mathrm{h.\,c}\\
H_{dt} &= \frac{1}{2}t_d\Phi^\dagger_L\tau_z\Phi_R + \mathrm{h.\,c}
\end{aligned}$$

Here, $\tau$ and $\sigma$ denote Pauli matrices in particle-hole, and spin space, respectively. The superconducting gaps, $\Delta_{L/R}$, as well as the dot-lead, and interdot tunnel couplings, $t_{L/R}$ and $t_d$, are all assumed to be real. Performing the following gauge transformations:

$$\Psi_{ik}(t) \to \bar{\Psi}_{ik}(t)e^{i\mu_i\tau_z t/\hbar}, \qquad (2)$$

$$\Phi_i(t) \to \bar{\Phi}_i(t)e^{it\mu_i\tau_z/\hbar}, \qquad (3)$$

the chemical potentials, $\mu_i$, are gauged away from $H_s$ and $H_d$ at the cost of making the interdot tunnel coupling time dependent:

$$H_{dt} \to \frac{1}{2}t_d\bar{\Phi}^\dagger_L e^{ieV\tau_z t/\hbar}\tau_z\bar{\Phi}_R + \mathrm{h.\,c} \qquad (4)$$

with $eV = \mu_R - \mu_L$. For $t_d = 0$, the left/right retarded $4 \times 4$ Nambu Green functions are readily found as

$$G^R_{0i}(\omega) = \left(\omega + i\bar{\eta}_i - \epsilon_d\tau_z - B_i\sigma_i - \Sigma^R_{ii}(\omega)\right)^{-1}, \qquad (5)$$

with tunnelling self-energy

$$\Sigma_{ii}^R(\omega) = -\Gamma_i \frac{\omega + \Delta_i \tau_x}{\sqrt{\Delta_i^2 - (\omega + i\eta_s)^2}}, \tag{6}$$

and where a phenomenological relaxation rate, $\bar{\eta}_i$, has been added to describe intrinsic relaxation on the dots. In principle, $\bar{\eta}_i$ could be frequency dependent but we choose to model it as a constant, tacitly associating it with a weak tunnel coupling between the dot and a wide-band normal metallic density of states. The tunnelling rates in the self-energy are given by $\Gamma_i = \pi\nu_i t_i^2$ with $\nu_i$ denoting the normal state density of states of the left/right lead, and the local mean-field spin directions are chosen in terms of Pauli matrices $\sigma_L = \sigma_z$ and $\sigma_R = \sigma_x$. A Dynes parameter, $\eta_s$, is included merely to allow for a numerical evaluation of the BCS coherence peaks.

In the limit of $B_i, \Gamma_i \gg \Delta_i$ and at the particle-hole symmetric point, $\epsilon_i = 0$, the Green functions, $G_{0i}^R(\omega)$, have a sub-gap pole at

$$\omega_i = \Delta_i \frac{(B - i\bar{\eta}_i)^2 - \Gamma_i^2}{(B - i\bar{\eta}_i)^2 + \Gamma_i^2} \approx \Delta_i \frac{1 - \alpha_i^2}{1 + \alpha_i^2} - i\eta_i/2, \tag{7}$$

where the last approximation is valid for $\bar{\eta}_i \ll B_i,\ \Gamma_i$. Here $\alpha_i = \Gamma_i/B_i = 2\pi\nu_i t_i^2/U$ and $\eta_i = 8\bar{\eta}_i B_i \Delta_i \Gamma_i^2/(B_i^2 + \Gamma_i^2)^2$, allowing us to identify these poles as lifetime broadened YSR states [10]. In our calculations, we assume for simplicity that $\eta_L = \eta_R$ and find the corresponding $\bar{\eta}_i$, which we then use for all values of $\epsilon_i$ in Eq. (5). In effect, this means that the intrinsic relaxation of the subgap states depends only weakly on $\epsilon_i$, as observed also in the experiment.

Since each individual dot is assumed to be in equilibrium with its respective superconducting lead, its occupation is readily determined by the fluctuation-dissipation theorem, i.e. $G_{0i}^<(\omega) = \left(G_{0i}^A(\omega) - G_{0i}^R(\omega)\right) n_F(\omega)$, where the advanced Green function has been found as $G_{0i}^A(\omega) = \left[G_{0i}^R(\omega)\right]^\dagger$. Using these Green functions the interdot tunnelling current is determined (using standard Langreth rules) as

$$\begin{aligned} I(t) &= \frac{e}{i\hbar} \sum_\sigma \langle [H_{dt}(t), n_L(t)] \rangle = \frac{e}{i\hbar} \operatorname{Re} \operatorname{Tr} \left[ e^{i\mu\tau_z t/\hbar} \langle \bar{\Phi}_R(t) \bar{\Phi}_L^\dagger(t) \rangle \right] \\ &= \frac{e}{\hbar} \operatorname{Re} \operatorname{Tr} \left[ \tau_z M^R \circ \left( \Sigma_{LL}^R \circ G_{0L}^< + \Sigma_{LL}^< \circ G_{0L}^A \right) \circ M^A \right], \end{aligned} \tag{8}$$

with $\circ$ denoting convolution in time-domain, $A \circ B = \int_{-\infty}^{\infty} dt' A(t, t') B(t', t'')$. The compo-

nents are defined as follows,

$$\Sigma^X_{LL}(t,t') = t_d^2 e^{i\mu\tau_z t/\hbar}\tau_z G^X_{0R}(t,t')\tau_z e^{-i\mu\tau_z t'/\hbar} \tag{9}$$

$$M^X(t,t') = \delta(t-t') + \Sigma^X_{LL}\circ G^X_{0L}\circ M^X, \tag{10}$$

with $X\in\{R,A,<\}$ for $\Sigma$ and $X\in\{R,A\}$ for $M$.

In our current framework only $H_{dt}$ is time dependent and periodic in $T = 2\pi/\Omega$ with $\Omega = eV/\hbar$.It is therefore convenient to define the following set of transformations,

$$G^X(t,\omega) = \int_{-\infty}^{\infty} dt' e^{i\omega(t-t')}G^X(t,t') \;\Leftrightarrow\; G^X(t,t') = \frac{1}{2\pi}\int_{-\infty}^{\infty} d\omega G^X(t,\omega)e^{-i\omega(t-t')} \tag{11}$$

$$G^X_n(\omega) = \frac{|\Omega|}{2\pi}\int_0^T dt e^{in\Omega t}G^X(t,\omega) \quad\Leftrightarrow\; G^X(\omega,t) = \sum_n G^X_n(\omega)e^{-in\Omega t}, \tag{12}$$

leading to the following representation of Green functions as matrices in Floquet space:

$$G^X_{nm}(\omega) = G^X_{n-m}(\omega + m\Omega). \tag{13}$$

This transformation conveniently maps a convolution in time domain to a matrix product in Floquet space, i.e.

$$C(t,t'') = \int_{-\infty}^{\infty} dt' A(t,t')B(t',t'') \;\Leftrightarrow\; C_{nm}(\omega) = \sum_l A_{nl}(\omega)B_{lm}(\omega), \tag{14}$$

.

Writing the current operator in Floquet space (i.e. as a Fourier series), $I(t) = \sum_n I_n e^{-in\Omega t}$, the measured DC component is now readily obtained as,

$$I_0 = \frac{e}{h}\int_{-\infty}^{\infty} d\omega\,\mathrm{Tr}\left[\tau_z \boldsymbol{M^R}\left(\boldsymbol{\Sigma^R_{LL}G^<_{0L}} + \boldsymbol{\Sigma^<_{LL}G^A_{0L}}\right)\boldsymbol{M^A}\right]_{00}, \tag{15}$$

with symbols in bold expressed as Floquet matrices evaluated at energy $\omega$. The index 00 refers to initial and final floquet component while trace is over Nambu space. In Floquet space $\boldsymbol{G^X_{0L}} = \delta_{nm}G_{0L}(\omega + m\Omega)$ is diagonal, while $\boldsymbol{\Sigma^X_{LL}}$ is a block-tridiagonal matrix of the form,

$$\Sigma^X_{LL,nm} = \begin{pmatrix} \delta_{n,m}t_d^2 G^X_{0R,11}(\omega+n\Omega) & -\delta_{n,m-2}t_d^2 G^X_{0R,12}(\omega+n\Omega) \\ -\delta_{n,m+2}t_d^2 G^X_{0R,21}(\omega-n\Omega) & \delta_{n,m}t_d^2 G^X_{0R,22}(\omega-n\Omega)\end{pmatrix}, \tag{16}$$

where entrance refers to particle-hole component such that $G^X_{0R,ij}(\omega)$ is a $2\times2$ matrix in spin space of the $ij^{\text{th}}$ particle-hole entrance in the original $4\times4$ Nambu Green functions. In Floquet space, the Dyson equation for $\boldsymbol{M^R}$ reduces to the matrix equation

$$\boldsymbol{M^R} = \boldsymbol{1} + \boldsymbol{\Sigma^R_{LL}G^R_{0L}M^R} = \left[\boldsymbol{1} - \boldsymbol{\Sigma^R_{LL}G^R_{0L}}\right]^{-1}, \tag{17}$$

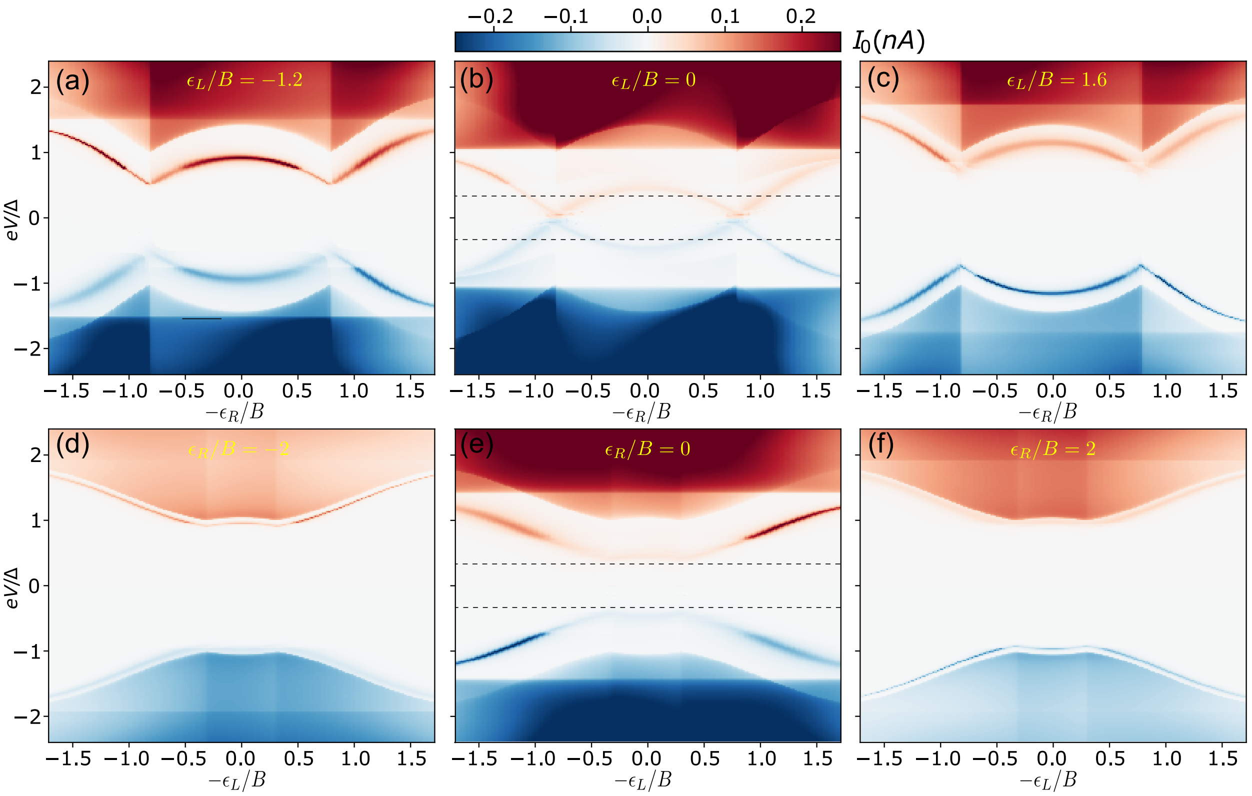


FIG. S3. (a-f) Calculation of current as a function of bias and dot tuning $\epsilon_i$. Dot tuning is chosen to match linecuts in Fig. 3 in the main article. Dotted lines in (b) and (e) indicate the bias range shown in Figs. S4. Plots are made with parameters [11] and including two Floquet sidebands.

which is solved by numerical inversion using a truncated Floquet space, including enough sidebands to ensure sufficient convergence. The advanced component is obtained as $\boldsymbol{M^A} = \left[\boldsymbol{M^R}\right]^\dagger$. Solving Eq. (15), including only two sidebands (truncation to $5\times5$ Floquet matrices with $-2 \leq n \leq 2$), is enough to ensure convergence of the salient features observed in Fig. S3. In the low-bias region, however, additional fine structure, requiring more sidebands to be included, will be in investigated further in subsection S2 A.

In comparison to the experimental data, these calculations show large changes in width of the $eV = E_L + E_R$ peaks for different dot tunings, and the sharp features in current will therefore dominate the non-linear conductance, $dI_0/dV$. These differences are smeared out by an additional $P(E)$ broadening, reflecting the inevitable fluctuations in bias voltage, which are present in realistic circuits. This is implemented as the convolution, $I(V) = \int_{-\infty}^{\infty} dE I_0(E)P(E-V)$, with a gaussian distribution, $P(E) = e^{-E^2/2\sigma^2}/\sqrt{2\pi}\sigma$, with a spread $\sigma = 0.04\Delta \approx 6\,\mu eV$, chosen to make the width of conductance peaks similar to observed

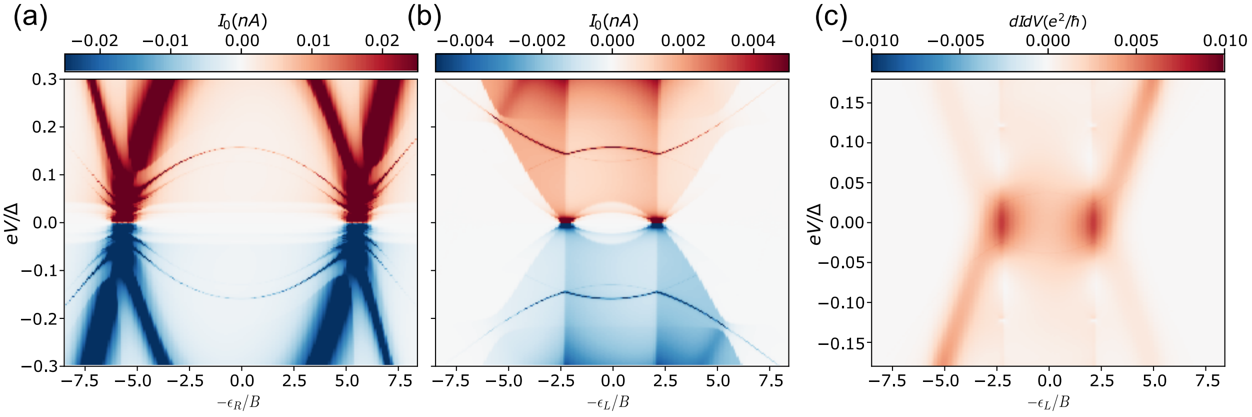


FIG. S4. Calculations of low bias current with (a) $\epsilon_L = 0$ and (b) $\epsilon_R = 0$ corresponds to (b) and (e) in Fig. S3. (c) Conductance obtained by convolving and differentiating current in (b). All plots are with parameters [11]. and using 4 sidebands.

peak width in experiment. The plots presented in Fig. 4 in the main text are obtained from such $P(E)$-broadening of the plots shown in Figs. S3 along the bias axis followed by numerical differentiation to obtain the conductance.

### A. Low bias features

In this subsection we investigate the effects of multiple Andreev reflections for small bias, for which it is necessary to include more Floquet bands to assure convergence. In Figs. S4 (a) and (b) we show low-bias current calculations using four sidebands. This is enough to observe a number of sharp lines of current at integer fractions of the previously described features, i.e. $eV = (E_{L/R} + \Delta_{R/R})/n$ (cf. also Ref. 6) and $eV = (E_L + E_R)/n$ 7). As the areas under these current peaks are much smaller than for the $n = 1$ peaks at higher bias, the subsequent $P(E)$ broadening used above renders these low-bias features unobservable in the experiment. In Fig. S4 (b) we also identify current plateaus starting at $eV = E_{L/R}$, which we identify as the weak metallic density of states (DOS), which we use to model the intrinsic relaxation, probing the subgap state [6, 12]. In Fig. S4 (c) we show the nonlinear conductance obtained by $P(E)$-broadening and subsequent differentiation of the current in Fig. S4 (b). This is seen to smear out the sharp MAR signal and leaves a marked set of conductance peaks of height comparable to those observed in the experimental data shown in Figs. S2. The fact that the weak metallic DOS, which we have included as a model for

the intrinsic relaxation needed to describe the $eV = E_L + E_R$ peaks in experiment, also yields a consistent description of the weak replicas crossing zero in experiment suggests that the metallic DOS is a real feature of the experiment rather than a just a simple means of modelling relaxation.

### B. Multigap model

In the experiment, multiple higher-lying replicas of the $eV = E_{L/R} + \Delta_{R/L}$ feature are observed. In this subsection we illustrate how such replicas can arise from including multiple subbands in the proximitized InAs wires comprising the leads. Modelling the DOS of each of the two superconducting leads ($i = L, R$) by a sum of BCS peaks for each subband (indexed here by $j = 1, 2, 3, 4, 5$) with each their gap, $\Delta_{ij} \in \{1.0, 1.1, 1.2, 1.3, 1.4\}\Delta$ with $\Delta = 0.14$meV, the left and right tunnelling self-energies are readily found as,

$$\Sigma^R_{ii}(\omega) = -\Gamma_i \sum_j \frac{\omega + \Delta_{ij}\tau_x}{\sqrt{\Delta_{ij}^2 - (\omega + i\eta_s)^2}}. \tag{18}$$

This self-energy is then used to compute the left, and right Green functions so as to obtain the current using Eq. (15).

Results of this calculations are shown in Fig. S5, which corresponds linecut 2 in Fig. 3 in the main text. One observes replicas of the $eV = E_{L/R} + \Delta_{R/L}$ feature appearing as individual subband BCS peaks probe the opposing subgap state. At the same time, only one subgap state is formed on either side, yielding only a single $eV = E_L + E_R$ feature. We note that earlier calculations using the zero-bandwidth approximation have shown similar results [13]. Interestingly, as the bound state acquires quasiparticle spectral weight from 5 different subbands, their individual BCS peaks remain relatively sharp, unlike for a single subband for which the YSR state depletes its BCS peak altogether. These residual BCS peaks in a multi-subband system therefore lead to enhanced MAR processes and the $eV = E_{L/R} + \Delta_{R/L}$ features exhibit negative differential conductance. All these features of course depend on the tunnelling rates of the individual subbands, all of which were here assumed to be equal for simplicity.

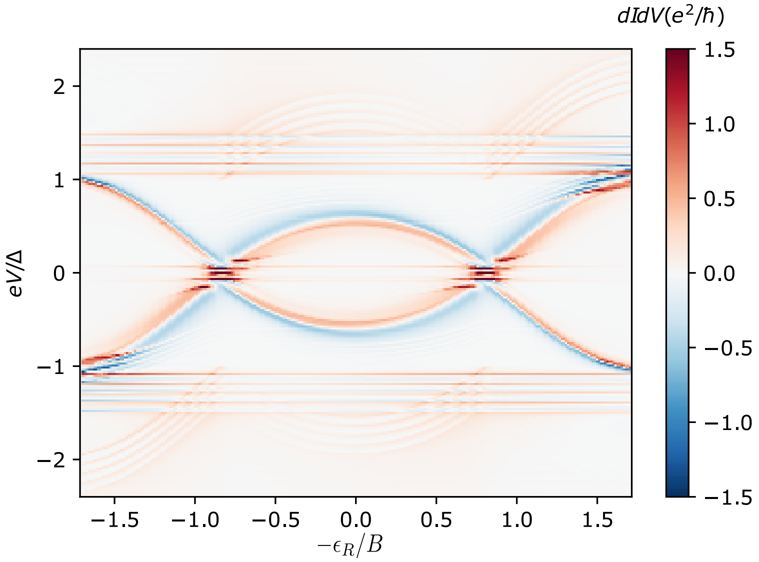


FIG. S5. Calculation of conductance using Eq. (18) as a function of energy tuning with $\epsilon_L = 0$. Calculations are truncated at two Floquet sub-bands so results close to zero $eV < 0.2\Delta$ could contain additional contributions. With Parameters from [11] but with $\Gamma_L = 1.3$ and $\Gamma_R = 0.8$ in units of $\Delta$.

## S3. MASTER EQUATIONS FOR SUBGAP STATE TRANSPORT

To obtain a more complete understanding of the relaxational transport between two subgap states at resonance, we support the Green function analysis above by a separate calculation of the current using master equations of the Lindblad form for the boundstate density matrix (cf. e.g. Refs. [14, 15], and references therein). This approach follows the procedure used in ref. [16] to describe subgap transport with intrinsic relaxation, but here expanded to also include relaxation by Andreev reflections.

With the simplifying assumption that both ground state and excited state of each subgap system are non-degenerate (singlets) the full Hilbert space of the system is spanned by $|0,0\rangle$, $|0,1\rangle$, $|1,0\rangle$ and $|1,1\rangle$ where left (right) number refers to left (right) subgap states state, denoting ground state and excited state by 0 and 1, respectively. In terms of the bias-voltage detuning, $e\delta V = eV - E_L - E_R$, the coherent dynamics of the subgap system is captured by the $2\times 2$ Hamiltonian of the even-parity subspace $\{|0,0\rangle, |1,1\rangle\}$,

$$H_{2\times 2} = \begin{pmatrix} -e\delta V/2 & \gamma_e \\ \gamma_e & e\delta V/2 \end{pmatrix} \tag{19}$$

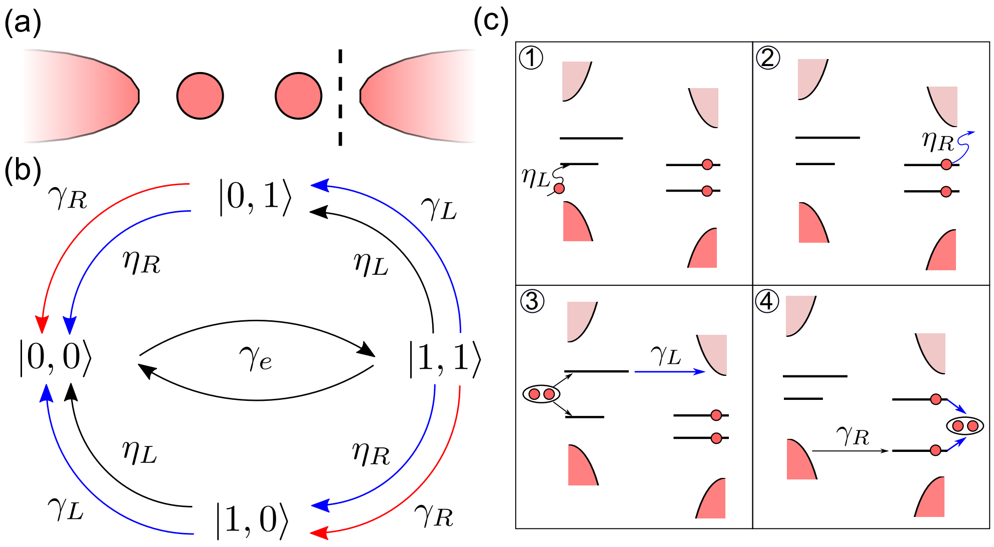


FIG. S6. (a) System schematic. Dashed line indicates threshold for current. (b) Diagram of transport dynamics. Black lines transfer no electrons, while blue lines transfer one electron and red lines transfer two electrons. (c) Schematic drawing of relaxation processes where blue lines indicate when an electron pass the barrier in (a).

with tunnelling amplitudes for transitions $|0,0\rangle \leftrightarrow |1,1\rangle$ denoted by $\gamma_e$. This amplitude is given by $\gamma_e = v_L u_R t_d$, if the left hole peak is aligned with the right electron peak ($\delta V = 0$) as in Fig. S6(c), and by $\gamma_e = u_L v_R t_d$ in the opposite case for negative bias ($eV = -E_L - E_R$). By themselves, these coherent transitions do not carry any net current, and for this we need to include incoherent relaxation processes. We include four independent relaxation rates, $\eta_i$ and $\gamma_i$ for $i \in \{L, R\}$ shown in Figs. S6 (c), where $\eta_i$ describes intrinsic relaxation processes occurring in each lead independently, while $\gamma_i$ describe relaxation through Andreev reflection employing the density of continuum states in opposing leads .

We choose to calculate the current as the rate of electrons leaving the right subgap state and entering the right lead. With this definition, $\eta_R$ and $\gamma_L$ both transfer one electron while $\gamma_R$ transfers two electrons as shown in Fig. S6 (c). The current can then be written as,

$$I = 2\pi\frac{e}{h}\left[(2\gamma_R + \gamma_L + \eta_R)P_{11} + (2\gamma_R + \eta_R)P_{10} + \gamma_L P_{01}\right], \tag{20}$$

where $P_i = \rho_{ii}$ is the occupation probability of state $|i\rangle$, found as the diagonal elements, $\rho_{ii}$, of the $4 \times 4$ density matrix operating in the full Hilbert space spanned by states $\{|0,0\rangle, |0,1\rangle, |1,0\rangle, |1,1\rangle\}$. In order to determine the density matrix, the total relaxation

rates on either side, $\Lambda_i = \eta_i + \gamma_i$, are included via jump operators

$$L_1 = \sqrt{\Lambda_L}\,|0,1\rangle\langle 1,1|\,,\;\; L_2 = \sqrt{\Lambda_R}\,|1,0\rangle\langle 1,1|\,, \tag{21}$$

$$L_3 = \sqrt{\Lambda_L}\,|0,0\rangle\langle 1,0|\,,\;\; L_4 = \sqrt{\Lambda_R}\,|0,0\rangle\langle 0,1|\,, \tag{22}$$

whereby the density matrix is found by solving the Lindblad master equation:

$$\hbar\frac{d\rho}{dt} = i\,[H_{2\times 2},\rho] + \sum_i \left( L_i\rho L_i^\dagger - \frac{1}{2}\{L_i^\dagger L_i,\rho\}\right), \tag{23}$$

where $\{\cdot,\cdot\}$ denotes an anticommutator. Rewriting this equation, and keeping only off-diagonal terms for $|1,1\rangle$ and $|0,0\rangle$ where tunnel coupling builds coherence, we obtain,

$$\begin{aligned}\hbar\frac{d\rho}{dt} = i\,[H_{2x2},\rho] - (\Lambda_R+\Lambda_L)P_{11}\,|1,1\rangle\langle 1,1| + (\Lambda_R P_{10}+\Lambda_L P_{01})\,|0,0\rangle\langle 0,0| \\ + (\Lambda_L P_{11} - \Lambda_R P_{01})\,|0,1\rangle\langle 0,1| + (\Lambda_R P_{11} - \Lambda_L P_{10})\,|1,0\rangle\langle 1,0| \\ - \frac{(\Lambda_R+\Lambda_L)}{2}\left(\rho_{11,00}\,|1,1\rangle\langle 0,0| + \rho_{00,11}\,|0,0\rangle\langle 1,1|\right),\end{aligned} \tag{24}$$

which we solve for the steady state occupation numbers by enforcing $\frac{d\rho}{dt} = 0$ and $\sum_i P_i = 1$. This yields $P_{01} = \frac{\Lambda_L}{\Lambda_R}P_{11}$, $P_{10} = \frac{\Lambda_R}{\Lambda_L}P_{11}$ and

$$P_{11} = \frac{\gamma_e^2}{\gamma_e^2\frac{(\Lambda_L+\Lambda_R)^2}{\Lambda_L\Lambda_R} + \frac{(\Lambda_L+\Lambda_R)^2}{4} + e^2\delta V^2}. \tag{25}$$

From this, we obtain the expression for the current presented in the main text describing a Lorentzian peaked around $eV = E_L + E_R$:

$$I = 2\pi\frac{e}{h}\frac{\gamma_e^2\left[\Lambda_L\left(1+\frac{\gamma_R}{\Lambda_R}\right) + \Lambda_R\left(1+\frac{\gamma_L}{\Lambda_L}\right)\right]}{\gamma_e^2\frac{(\Lambda_L+\Lambda_R)^2}{\Lambda_L\Lambda_R} + \frac{(\Lambda_L+\Lambda_R)^2}{4} + e^2\delta V^2}. \tag{26}$$

If we extract the bound state energies, $E_i$, and the effective relaxation rates, $\eta_i$, from the denominator in Eq. (5), in addition to the coherence factors $u_i$ and $v_i$, we can calculate the Andreev mediated relaxation rate by Fermi's golden rule:

$$\gamma_L = \pi u_L^2 t_d^2 d_R(2E_L + E_R) \;\text{ and }\; \gamma_R = \pi v_R^2 t_d^2 d_L(-2E_R - E_L), \tag{27}$$

for positive biases where the left hole peak is aligned with the right electron peak. For the opposite case, left electron sector aligned with right hole sector, let $u_i \to v_i$, $v_i \to u_i$ and $E_i \to -E_i$. In Fig. S7 we compare results obtained from the master equation and the Floquet Keldysh Green functions, respectively. Apart from the continuum, which is not included in the former, this demonstrates an excellent match between the two different methods when it comes to describing the relaxational current peaks at $eV = \pm(E_L + E_R)$.

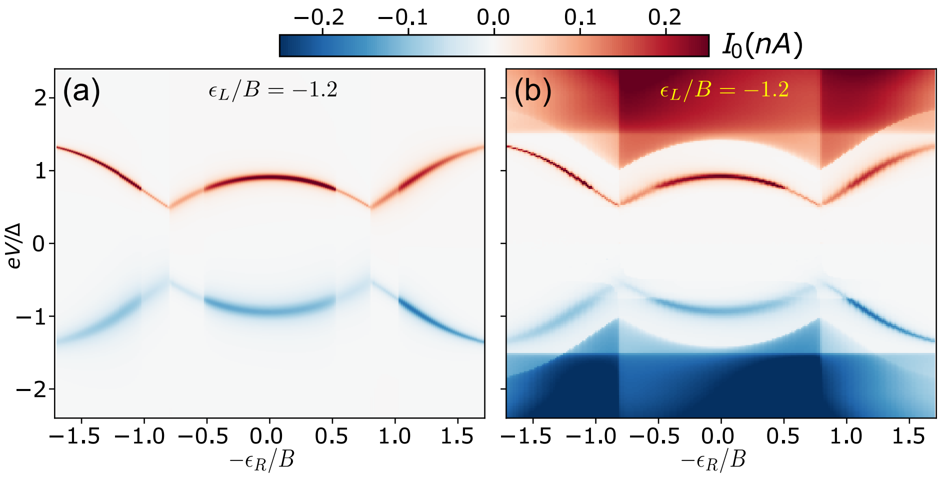


FIG. S7. Calculation of current. a) is calculated using Eq. (26) and b) using Eq. (15) both using the spin polarized mean-field with parameters [11].

### A. Conductance asymmetry

Both data and theory show a notable bias asymmetry in conductance near $eV = \pm(E_L + E_R)$. In the limit, $\eta_i \gg t_d$, where current can be calculated using Fermi's golden rule, we expect this asymmetry to reflect directly the frequency asymmetry of the underlying spectral function, which is present for $u_i \neq v_i$ away from the particle-hole symmetric point. As the width of conductance features is provided by $P(E)$-broadening, the interesting quantity to compare is the integral of Eq. (26), since this area under the current peak determines the conductance. In the limit of $\eta_i \gg \gamma_i$, $\gamma_e$ we find this area to be

$$A_I = 4\pi^2 \frac{e}{h} \gamma_e^2. \tag{28}$$

Since $\gamma_e^2$ is proportional to the spectral weight of the aligned peaks ($\gamma_e^2 \propto v_L^2 u_R^2$ for left hole aligned with right electron sector) the asymmetry of this area matches that of the underlying spectral functions, and the bias asymmetry is set by the ratio $v_L^2 u_R^2 / u_L^2 v_L^2$. In the opposite limit where $t_d \gg \eta_i$, we instead obtain

$$A_I = 4\pi^2 \frac{e}{h} \frac{\gamma_e^2}{\sqrt{\frac{\gamma_e^2}{\gamma_L \gamma_R} + \frac{1}{4}}} \tag{29}$$

for which it is the factor $v_L^2 u_R^2 / u_L^2 v_L^2$ in competition with $\pi^2 t_d^2 d_L(2E_L + E_R) d_R(-2E_R - E_L)$, which determines the bias asymmetry This complicated relation strongly depends on the energy levels $\epsilon_i$ (set by the gate voltages in the experiment) which determine the coherence

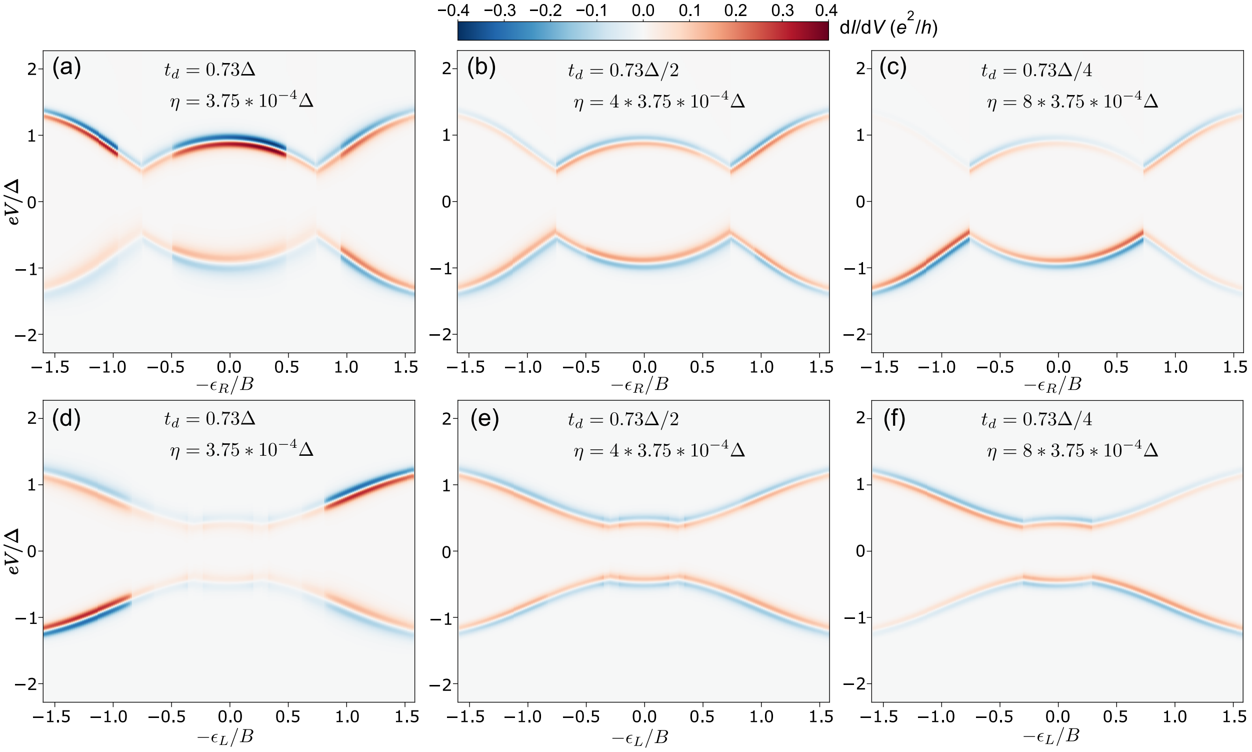


FIG. S8. Calculation of conductance using Eq. (26) with a $P(E)$ convolution for three different values of $\eta_i$. (a-c) are with $\epsilon_L/B = -8.4$ and (d-f) are with $\epsilon_R/B = 0$. Other parameters are from [11]. Plots (c) and (f) correspond to the Fermi's golden rule limit.

factors $u_i$, $v_i$, and for the parameters extracted for the present experiment the marked conductance asymmetry is opposite to that of the Fermi's golden rule limit, as seen in Fig. S8, indicating a relatively weak intrinsic relaxation rate, $\eta_i \ll t_d$.

### B. Singlet-to-doublet Master Equations

So far, we have simplified the transport calculations by using spin polarized mean field theory, which has lead to non-degenerate sub-gap states. There is, however, no reason to believe that spin rotational invariance should be broken in this system and each of the (left/right) sub-gap systems are therefore expected to comprise a singlet and a doublet. The total number of states for the two-subgap-state system is then 9, instead of 4, with states $|S,S\rangle$, $|S,\sigma\rangle$, $|\sigma,S\rangle$ and $|\sigma,\sigma'\rangle$ with $\sigma \in \{\uparrow,\downarrow\}$ and left/right position denoting left/right subgap state. In this final section, we extend the master equations to deal with the full spin-degenerate problem. This allows us to assess the potential shortcomings of the spin-

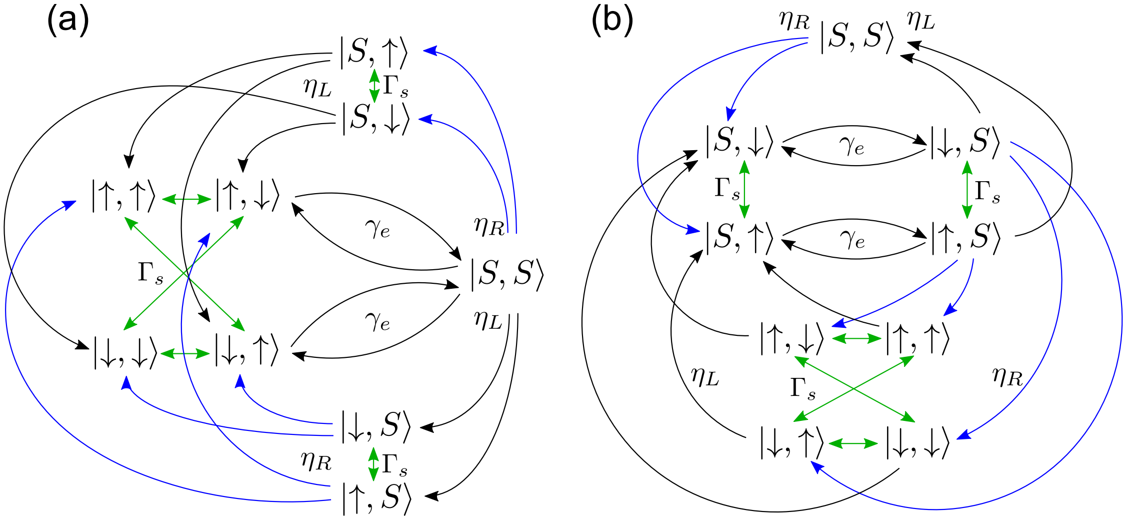


FIG. S9. Schematic of transport dynamics. (a) is for the $|\sigma,\sigma'\rangle$ ground state while (b) is for the $|S,\sigma\rangle$ ground state. Black lines indicate processes that transfer no electrons while blue lines indicate processes that transfer a single electron. Green lines indicate spin-flip processes that does not change fermion parity. Lines with $\gamma_e$ we treat as coherent processes the rest are modelled as jump operators. To obtain the corresponding diagram for the $|S,S\rangle$ and $|\sigma,S\rangle$ ground state flip direction of all $\eta_i$ lines in (a) and (b) correspondingly.

polarized mean field approximation in the transport calculations presented above and in the main text.

Our approach follows the template from the singlet-to-singlet master equation. For simplicity, we assume that relaxation by Andreev reflection can be ignored, i.e. $\gamma_i \approx 0$, corresponding to the blue regime in Fig. 1 (b). We assume that relaxation occurs independently on either side, such that a doublet $|\sigma\rangle$ relaxes to singlet state $|S\rangle$, while a singlet relaxes either to $|\uparrow\rangle$ or $|\downarrow\rangle$. Both processes are assumed to take place with rates $\eta_i$. As such, singlet states experience a higher total relaxation rate than doublet states. In Fig. S9 (a) we show a heuristic diagram of the governing dynamics when both subgap states are in a doublet ground state, $|\sigma,\sigma'\rangle$, with bias $eV = E_L + E_R + e\delta V$ such that coherent tunneling can drive transitions $|\uparrow,\downarrow\rangle$, $|\downarrow,\uparrow\rangle \leftrightarrow |S,S\rangle$. The coherent part is described by the Hamiltonian,

$$H_{DD-SS} = \begin{pmatrix} e\delta V/2 & \gamma_e & -\gamma_e \\ \gamma_e & -e\delta V/2 & 0 \\ -\gamma_e & 0 & -e\delta V/2 \end{pmatrix} \tag{30}$$

where the first entrance is the $|S,S\rangle$ state and second and third are $|\uparrow,\downarrow\rangle$ and $|\downarrow,\uparrow\rangle$, respectively. In this relaxation scheme, the system may end up in triplet state, $|\sigma,\sigma\rangle$, which will block the current. To lift this Pauli spin blockade, we include a spin-flip rate, $\Gamma_s$, which flips the spin of the subgap state without changing fermion parity. These are included as Markovian jump operators, just as for the quasiparticle relaxation, and are represented by green arrows in Fig. S9.

The Lindblad master equation now takes the following form:

$$\hbar\frac{d\rho}{dt} = i\left[H_{DD-SS},\rho\right] + \sum_i \left[L_i\rho L_i^\dagger - \frac{1}{2}\{L_i^\dagger L_i,\rho\}\right], \tag{31}$$

where $\rho$ is a $9\times 9$ density matrix. For each arrow in Fig. S9 (indexed by $i$ in the summation in Eq. (31)) pointing from state $l$ to a state $k$, we include a jump operator $L=\sqrt{X}\,|k\rangle\,\langle l|$ with rate $X$. Since only the $3\times 3$ block of Eq. (30) builds coherence, we can set all other non-diagonal components to zero. Solving the diagonal part of the master equation for the non-coherent part allows one to simplify the remaining master equation to a $3\times 3$ matrix equation, $\hbar\dot\rho = i\left[H_{DD-SS},\rho\right] + M$, with $M$ given by

$$M_{DD} = \begin{pmatrix} -2\eta_T\rho_{11} & -(\eta_T+\Gamma_s)\rho_{12} & -(\eta_T+\Gamma_s)\rho_{13} \\ -(\eta_T+\Gamma_s)\rho_{21} & \eta_T\rho_{11} & -2\Gamma_s\rho_{23} \\ -(\eta_T+\Gamma_s)\rho_{31} & -2\Gamma_s\rho_{32} & \eta\rho_{11} \end{pmatrix}, \tag{32}$$

for doublet-doublet ground state, and

$$M_{SS} = \begin{pmatrix} 2c\eta_T\rho_{22} & -(\eta_T/2+\Gamma_s)\rho_{12} & -(\eta_T/2+\Gamma_s)\rho_{13} \\ -(\eta_T/2+\Gamma_s)\rho_{21} & -c\eta_T\rho_{22} & -(\eta_T+2\Gamma_s)\rho_{23} \\ -(\eta_T+\Gamma_s)\rho_{31} & -(\eta_T+2\Gamma_s)\rho_{32} & -c\eta_T\rho_{22} \end{pmatrix}, \tag{33}$$

for singlet-singlet ground state. Here $\eta_T = \eta_L + \eta_R$ and $c = (\eta_T + 2\Gamma_s)/(\eta_T + 4\Gamma_s)$, and the state indices on $\rho$ have been defined as $SS = 1$, $\uparrow\downarrow = 2$ and $\downarrow\uparrow = 3$. Spin rotational invariance dictates that $\rho_{22} = \rho_{33}$. Solving for the normalized ($\mathrm{Tr}[\rho] = 1$) steady state ($\dot\rho = 0$) density matrix, and counting transported electrons from the $\eta_R$ process, similar to Eq. (20), we obtain the following currents for the different ground state configurations

$$I_{DD} = 2\pi\frac{e}{h}\frac{\gamma_e^2\left(\eta_T+2\Gamma_s\right)}{e^2\delta V^2 + \left(\eta_T+2\Gamma_s\right)^2 + \frac{1}{2}\gamma_e^2\frac{\eta_T+2\Gamma_s}{\eta_T}\left[3+\frac{\eta_T^2}{\eta_L\eta_R}+\frac{5}{2}\frac{\eta_T}{\Gamma_s}\right]}, \tag{34}$$

$$I_{SS} = 2\pi\frac{e}{h}\frac{2\gamma_e^2\left(\eta_T+\Gamma_s\right)}{e^2\delta V^2 + \frac{(\eta_T+\Gamma_s)^2}{4} + \gamma_e^2\frac{\eta_T+\Gamma_s}{\eta_T}\left[2+2\frac{\eta_L^2+\eta_R^2}{\eta_L\eta_R}+\frac{\eta_T}{\eta_T+\Gamma_s}\right]}. \tag{35}$$

Both formulas are Lorentzians and for $\Gamma_s \to 0$ we find $I_{DD} \to 0$ while $I_{SS}$ remains finite, reflecting the triplet blockade occurring if no spin-relaxation is present. In the case of a singlet-doublet ground state configuration, $|S,\sigma\rangle$, the $eV = E_L + E_R$ resonance drives transitions $|S,\sigma\rangle \leftrightarrow |\sigma,S\rangle$ as seen in Fig. S9. We setup up a master equation in a similar manner as before but now the system is composed of two symmetrical $2 \times 2$ blocks,

$$H_{SD-DS} = \begin{pmatrix} e\delta V/2 & \gamma_e \\ \gamma_e & -e\delta V/2 \end{pmatrix} \text{ and } M_{SD} = \begin{pmatrix} -\hat{\eta}\rho_{11} & -(\Gamma_s + \hat{\eta}/2)\rho_{12} \\ -(\Gamma_s + \hat{\eta}/2)\rho_{21} & \hat{\eta}\rho_{11} \end{pmatrix}, \quad (36)$$

in the basis $\{|S,\uparrow\rangle, |\uparrow,S\rangle\}$ and with $\hat{\eta} = \eta_R + 2\eta_L$. Similarly, the corresponding equation for a doublet singlet configuration, $|\sigma,S\rangle$, is obtained with $\hat{\eta} = 2\eta_R + \eta_L$. Utilizing again the spin-rotational invariance, we solve for the steady state density matrix and obtain the following current:

$$I_{SD} = 2\pi\frac{e}{h}\frac{\gamma_e^2(\bar{\eta} + \Gamma_s)}{e^2\delta V^2 + \frac{(\bar{\eta}+2\Gamma_s)^2}{4} + \gamma_e^2\frac{\bar{\eta}+2\Gamma_s}{2\bar{\eta}}\frac{\bar{\eta}^2}{\eta_L+\eta_R}}, \quad (37)$$

which again takes a Lorentzian form.

Next, we compare these results with experimental findings. A low-bias region, corresponding to the relaxational regime without Andreev mediated relaxation considered in this subsection, is clearly visible in linecuts 1, 2 and 5 presented in Fig. 3 of the main text. Following the $eV = E_L + E_R$ features through the gate voltage at which they change slope and the subgap system changes ground state, we do not observe any notable change in conductance. This observation enforces restrictions on parameters if current is indeed described by Eqs. (34), (35), and (37). The fact that we observe a finite conductance in the doublet-doublet sector means that $\Gamma_s$ cannot be zero. Overall, the experimental data are consistent with the assumption that $\gamma_e \gg \Gamma_s \gg \eta_L = \eta_L = \eta$, which ensures the lifting of Pauli spin blockade. As discussed in the previous subsection, the conductance is best described in terms of the area under the current peak, since this is independent of the $P(E)$ broadening. In the said limit of rates, one finds that

$$A_{SS} = 2\pi\frac{e}{h}\frac{2}{\sqrt{3}}\gamma_e\sqrt{\eta\Gamma_s}, \quad (38)$$

$$A_{DS} = 2\pi\frac{e}{h}\sqrt{\frac{2}{3}}\gamma_e\sqrt{\eta\Gamma_s}, \quad (39)$$

$$A_{DD} = 2\pi\frac{e}{h}\sqrt{\frac{2}{7}}\gamma_e\sqrt{\eta\Gamma_s}, \quad (40)$$

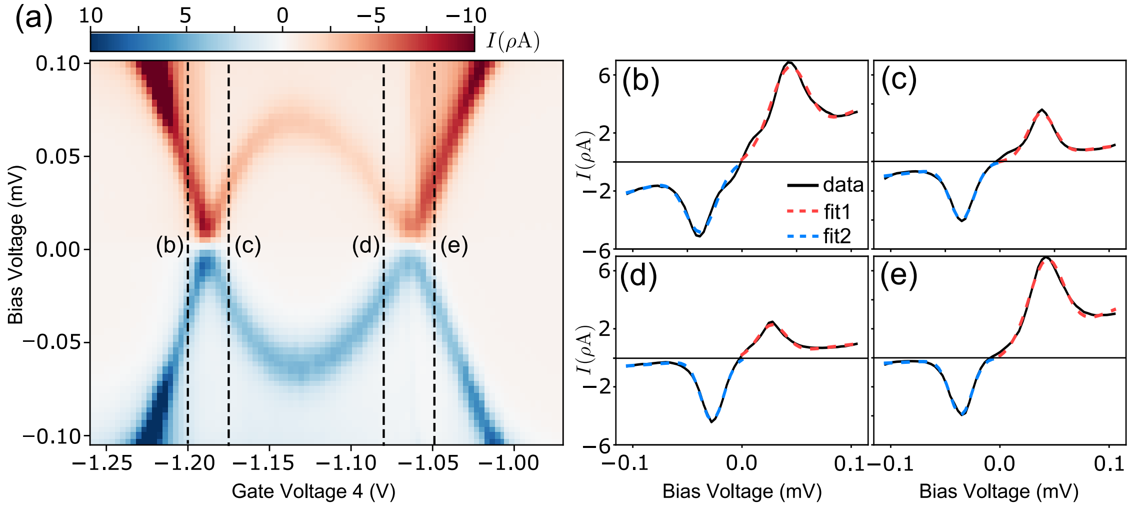


FIG. S10. (a) Experimentally acquired current as a function of bias and gate following linecut 2 in Fig. 3 of the main text. Dashed lines indicate cuts shown in (b-e). (b-e) Current as a function of bias for cuts on either side of the two phase transitions. The positive and negative peak are fitted by a Gaussian function plus a linear function accounting for tails.

with $A_{ij} = \int_{-\infty}^{\infty} d\delta V I_{ij}(\delta V)$. The fact that these three areas are equal up to a factor of approximately $\sqrt{2}$, and remain so in a wide parameter range without requiring fine tuning of rates is consistent with the experimental observation that the peak to peak conductance is largely constant across the phase transitions (changes in ground state).

To test this finding in greater detail, we consider again linecut 2 from Fig. 3 in the main text, for which $eV = E_L + E_R$ crosses zero two times within the regime where there is no Andreev mediated relaxation (cf. Fig. S10(a)). In Fig. S10(b-e) we show the results of fitting a Gaussian plus a linear function to the current peaks. From these fits, we extract the area under the positive and negative current peaks, excluding any contribution from the linear part, before and after the phase transition at the two crossings. Going from (b) to (c), or from (e) to (d), corresponds to a phase transition from a DS, to a DD ground state, as can be inferred from the charge diagram in Fig. 2 (b) of the main text. Comparing the area of the negative (positive) bias peaks in the DS sector with the area of the positive (negative) bias peak in the DD sector, we find that

$$\frac{A_{b+}}{A_{c-}} \approx 2.3, \quad \frac{A_{b-}}{A_{c+}} \approx 1.9, \quad \frac{A_{e+}}{A_{d-}} \approx 2.2, \quad \frac{A_{e-}}{A_{d+}} \approx 1.3, \tag{41}$$

where $A_{b+}$ denotes the area of the fitted Gaussian positive-bias peak at gate voltage indicated by the dashed line at (b), not including the contribution from the linear part of the fit, which

is required in order to fit the tails. In the small distance between (b) and (c), and (e) and (d), respectively, it is reasonable to assume that coherence factors, $u_i$ and $v_i$, are approximately constant, such that $\gamma_e$ remains constant. The ratio between expressions (39) and (40) should therefore be constant, i.e. $\frac{A_{DS}}{A_{DD}} = \sqrt{\frac{7}{3}} \approx 1.5$, slightly smaller then what we find by fitting.

In conclusion, we find that reinstalling spin-rotational invariance by including an odd-parity *doublet* ground state results in Lorenztian current peaks at the $eV = E_L + E_R$ resonance, just as for the singlet-singlet modeling building on the spin-polarized mean field approximation. Including the doublet state, however, it becomes apparent that the observation of relaxational peak-to-peak current in the doublet-doublet phase relies on a large spin-flip rate, $\Gamma_s \gg \eta$. At the same time, the observation of a stepwise change in conductance at the boundary between two different relaxation regimes requires strong inter-dot tunnelling, $\gamma_e \gg \Gamma_s$. Altogether, the hierarchy $\gamma_e \gg \Gamma_s \gg \eta_i$ with $\eta_L \approx \eta_R$, as employed in the main text, provides a consistent description of the experimental data. This includes the observation that the current peaks at $eV = E_L + E_R$ only change by a minor factor of approximately $\sqrt{2}$ when changing ground state.

[1] J. C. Estrada Saldaña, A. Vekris, G. Steffensen, R. Žitko, P. Krogstrup, J. Paaske, K. Grove-Rasmussen, and J. Nygård, Physical Review Letters (2018).

[2] J. C. Estrada Saldaña, A. Vekris, R. Žitko, G. Steffensen, P. Krogstrup, J. Paaske, K. Grove-Rasmussen, and J. Nygård, Phys. Rev. B **102**, 195143 (2020).

[3] I. Martin and D. Mozyrsky, Phys. Rev. B **90**, 100508 (2014).

[4] M. Ruby, F. Pientka, Y. Peng, F. von Oppen, B. W. Heinrich, and K. J. Franke, Phys. Rev. Lett. **115**, 087001 (2015).

[5] J. C. Cuevas, A. Martín-Rodero, and A. L. Yeyati, Phys. Rev. B **54**, 7366 (1996).

[6] A. Villas, R. L. Klees, H. Huang, C. R. Ast, G. Rastelli, W. Belzig, and J. C. Cuevas, Phys. Rev. B **101**, 235445 (2020).

[7] A. Villas, R. L. Klees, G. Morrás, H. Huang, C. R. Ast, G. Rastelli, W. Belzig, and J. C. Cuevas, Phys. Rev. B **103**, 155407 (2021).

[8] J.-d. Pillet, *Tunneling spectroscopy of the Andreev bound states in a carbon nanotube*, Ph.D. thesis, l'Université Pierre et Marie Curie (2011).

[9] M. Žonda, V. Pokorný, V. Janiš, and T. Novotný, Sci. Rep. **5**, 1 (2015).

[10] A. I. Rusinov, JETP Lett. **9**, 85 (1969), [Zh. Eksp. Teor. Fiz. **9**, 146 (1968)].

[11] Parameters used in plots: $\Delta_L = \Delta_R = \Delta = 0.14$meV, $B_L = B_R = 7$, $\Gamma_L = 6.65$, $\Gamma_R = 4.2$, $t_d = 0.73$, $\eta_L = \eta_R = 3.75 \times 10^{-4}$, $T = 10^{-3}$ and $\sigma = 0.04$ all in units of $\Delta$. The BCS density of states of the superconducting leads are broadened by $\eta_s = 10^{-6}\Delta$ for numerical reasons.

[12] A. Kumar, M. Gaim, D. Steininger, A. L. Yeyati, A. Martín-Rodero, A. K. Hüttel, and C. Strunk, Phys. Rev. B **89**, 075428 (2014).

[13] Z. Su, A. Zarassi, J.-F. Hsu, P. San-Jose, E. Prada, R. Aguado, E. J. H. Lee, S. Gazibegovic, R. L. M. Op het Veld, D. Car, S. R. Plissard, M. Hocevar, M. Pendharkar, J. S. Lee, J. A. Logan, C. J. Palmstrøm, E. P. A. M. Bakkers, and S. M. Frolov, Phys. Rev. Lett. **121**, 127705 (2018).

[14] H.-P. Breuer and F. Petruccione, in *The Theory of Open Quantum Systems* (Oxford University Press, Oxford, England, UK, 2007).

[15] D. Manzano, AIP Adv. **10**, 025106 (2020).

[16] H. Huang, C. Padurariu, J. Senkpiel, R. Drost, A. L. Yeyati, J. C. Cuevas, B. Kubala, J. Anker-

hold, K. Kern, and C. R. Ast, Nat. Phys. **16**, 1227 (2020).
